# Supplementary material for: Freezing, melting and the onset of glassiness in binary mixtures
Source: arXiv:2406.04921 ancillary file (2025-02-19)
Supplement: Supplementary file 1 [file supplement.pdf]

# Supplementary material for
# ”Freezing, melting and the onset of glassiness in binary mixtures”

Daniele Coslovich, Leonardo Galliano, Lorenzo Costigliola

## Contents

**1 Supplementary material** **1**
1.1 Simulation details . . . 1
1.2 Partial structure factors . . . 2
1.3 Additional details on the determination of the onset temperature . . . 3
1.4 Comparison of the methods to determine the onset temperature . . . 6
1.5 Stability of the onset temperature against statistical noise . . . 7
1.6 Composition-dependence of the onset temperature at different pressures . . . 8
1.7 Structural relaxation times along isotherms . . . 8
1.8 Oscillatory behavior of $tF_s'$ at short times . . . 9
1.9 Excess entropy scaling of relaxation times and diffusion coeffients . . . 10
1.10 Tabulated data . . . 11

**References** **16**

## 1 Supplementary material

### 1.1 Simulation details

We carried out most of the simulations and data analysis for a system of $N = 500$ particles using the `atooms` simulation framework [1]. Along **isobaric paths**, we performed equilibration runs by coupling the system to a Berendsen thermostat and a Berendsen barostat, integrating the equations of motion with a timestep $\delta t = 0.001$. The relaxation times for for the thermostat and the barostat were $\tau_T = 100\delta t$ and $\tau_P = 10^4\delta t$, respectively. We removed the drift of the center of mass every $2\times10^4$ steps. We performed the production runs with a Nose-Poincaré thermostat [2] using a timestep $\delta t = 0.001$ and a mass parameter $Q = 5$, fixing the volume to the average volume computed during the second half of the equilibration run. To obtain the onset temperatures shown in Fig. 2 of the main text we averaged the dynamic quantities over two independent trajectories for each state point. For the concentration $x = 0.2$, we performed 30 additional independent simulations for each state point along the isobar $P = 10.19$, to study the stability of the results against statistical noise, see Sec. **??**. Along **isochoric paths**, we performed simulations using the Nosé-Poincaré thermostat [2] with a timestep $\delta t = 0.002$ and a mass parameter $Q = 5$, for both equilibration and production runs. In all the simulations used to determine the onset temperature, we stopped the equilibration run when the root mean squared displacement of the largest particles reached 3; the subsequent production runs were twice as long. In the simulations used to determine the excess entropy we used a similar equilibration protocol, except along the isothermal paths, for which the target root mean squared displacement was interpolated between 16 at low density and 3 at the highest density along each isothermal path. At all state points and for each composition, we averaged the excess entropy data over two independent simulations.

We performed additional simulations for a larger system size, $N = 8000$, using RUMD [3]. In the simulations along **isochoric paths**, we controlled the temperature via a Nose-Hoover thermostat with relaxation time $\tau_{NH} = 0.2$ and a time step $\delta t = 0.0025$. We averaged the data from these $NVT$ simulations over 128 independent simulations at each state point. Along **isobaric paths**, we used the numerical integrator proposed in Ref. [4]. The relaxation times of the thermostat and barostat are $\tau_T = 0.4$ and

$\tau_P = 20$, respectively. Along both kinds of paths, we removed the drift of the center of mass every 100 steps. For each state point, the equilibration run comprised $2^{30}$ steps, regardless of pressure and temperature. We then performed a simulation in the NVT ensemble, fixing the density to the average one computed from the equilibration run. The production runs were started using independent starting configurations obtained from these $NVT$ simulations. From each configuration sampled in the $NVT$ ensemble as above, we carried out production runs in the $NVT$ ensemble for $2^{23}$ time steps.

## 1.2 Partial structure factors

To determine the relevant range of wave-vectors for the self intermediate scattering functions, we computed the partial structure factors $S_{\alpha\beta}(k)$ for different compositions $x$, slightly above the onset of glassiness. We keep the pressure constant at $P = 10.19$. From Fig. 1, we see that the position of the first peak of $S_{AA}(k)$ is close to $k = 7.2$ and that it is fairly insensitive to $x$. The $S_{BB}(k)$ structure factor has two sharp peaks, the first around 5.6, the other around 8, whose amplitude increases as $x$ increases towards 0.5. We found that the position of the peaks does not depend strongly on pressure, at least in the range of state conditions explored in this work, see Fig 2 for an example of such a calculation at $P = 30$. On basis of these observations, in the main text we focus on the range $k = 5-10$ for A-particles and $k = 4-8$ for B-particles.

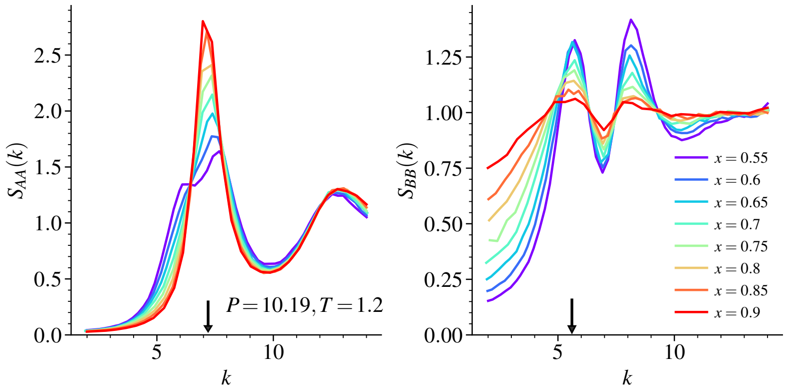


***Figure 1:*** *Partial structure factors $S_{AA}(k)$ (left) and $S_{BB}(k)$ (right) at the state point ($P = 10.19$, $T = 1.18$) for different compositions $x$. The vertical arrows are drawn at $k = 7.2$ and $k = 5.6$ in the left and right panel, respectively.*

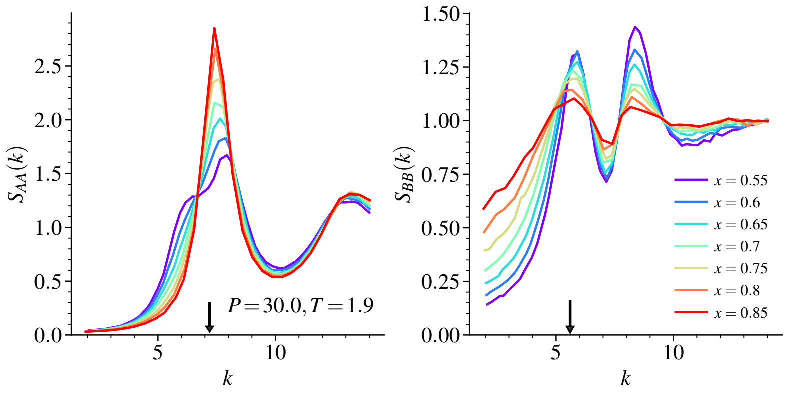


***Figure 2:*** *Partial structure factors $S_{AA}(k)$ (left) and $S_{BB}(k)$ (right) at the state point ($P = 30$, $T = 1.89$) for different compositions $x$. The vertical arrows are drawn at $k = 7.2$ and $k = 5.6$ in the left and right panel, respectively.*

### 1.3 Additional details on the determination of the onset temperature

In this section we provide additional details about the data underyling Fig. 2 of the main text and also include results for the B-particles.

Figures 3 to 6 display representative results for $F_s(k,t)$, $tF_s'(k,t)$, the order parameter $\delta$ and the Debye-Waller factor $f_s = F_s(k,t^*)$ at the canonical concentration $x = 0.2$. We show the results separately for the A-particles at $k = 7.2$ and for the B-particles at $k = 5.4$, close to the first sharp peaks in the corresponding partial structure factors. We see that the results for A- and B-particles are very similar to each other. While $\delta$ rises continuously at the onset temperature, the Debye-Waller factors $f_s$ jump discontinuously, as expected. We emphasize that the $F_s(k,t)$ shown here were averaged only over 2 independent trajectories, yet the results are consistent with those obtained in Fig. 1 of the the main text (30 trajectories). See also Sec. **??** below.

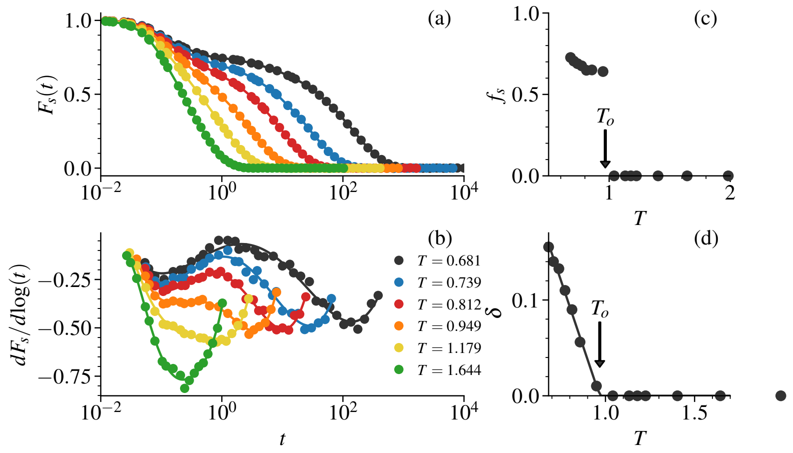


***Figure 3:*** *Overview of onset temperature determination for A-particles with concentration $x = 0.2$ at a pressure $P = 10.19$ for $N = 500$ particles: (a) $F_s(k,t)$ for selected temperatures around $T_o$ at $k = 7.2$; (b) derivatives $tF_s'(k,t)$ for the same temperatures as in (a); (c) Debye-Waller factor $f_s$ as function of $T$; (d) order parameter $\delta$ obtained from $tF_s'(k,t)$ as a function of $T$.*

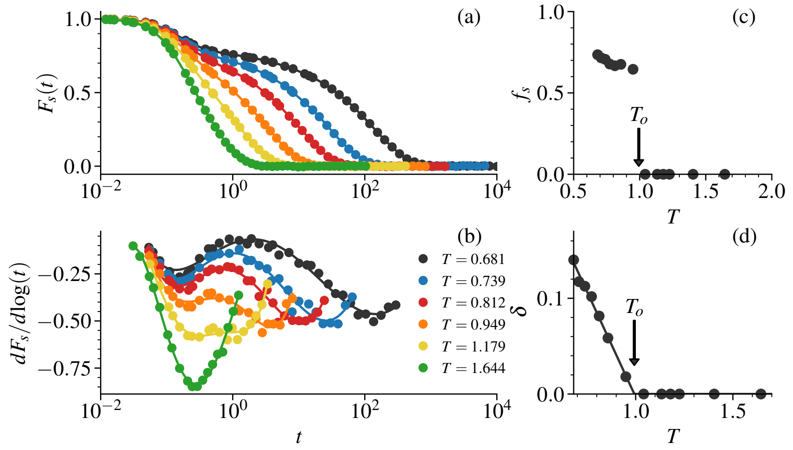


***Figure 4:*** *Overview of onset temperature determination for B-particles with concentration $x = 0.2$ at a pressure $P = 10.19$ for $N = 500$ particles: (a) $F_s(k,t)$ for selected temperatures around $T_o$ at $k = 5.4$; (b) derivatives $tF_s'(k,t)$ for the same temperatures as in (a); (c) Debye-Waller factor $f_s$ as function of $T$; (d) order parameter $\delta$ obtained from $tF_s'(k,t)$ as a function of $T$.*

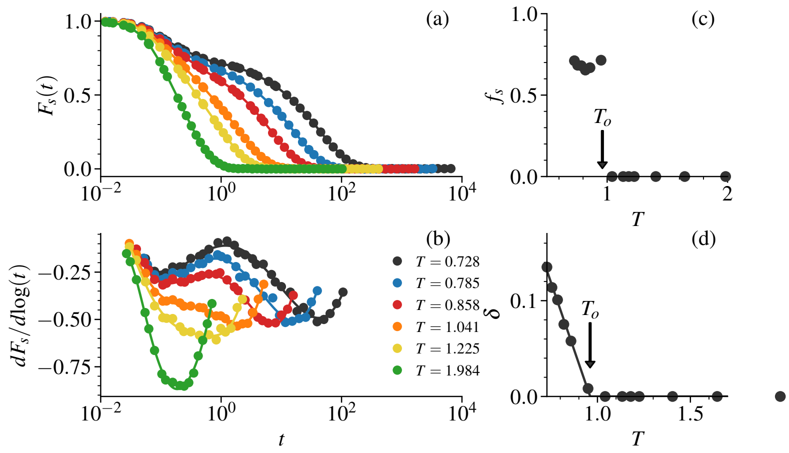


***Figure 5:*** *Overview of onset temperature determination for A-particles with concentration $x = 0.25$ at a pressure $P = 10.19$ for $N = 500$ particles: (a) $F_s(k,t)$ for selected temperatures around $T_o$ at $k = 7.2$; (b) derivatives $tF_s'(k,t)$ for the same temperatures as in (a); (c) Debye-Waller factor $f_s$ as function of $T$; (d) order parameter $\delta$ obtained from $tF_s'(k,t)$ as a function of $T$.*

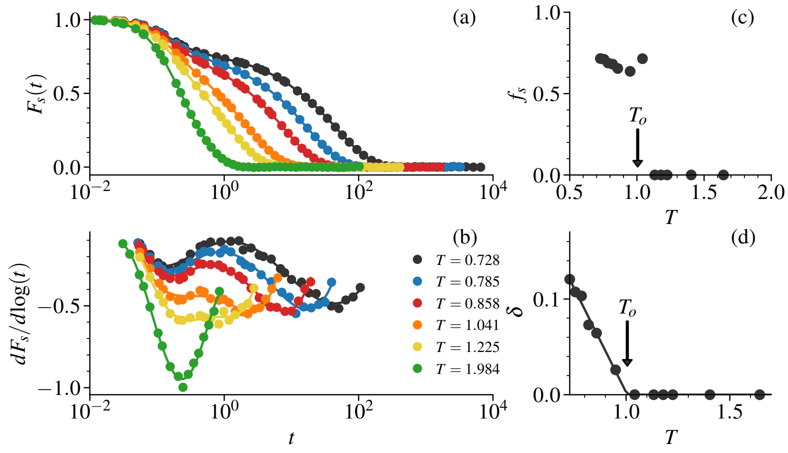


***Figure 6:*** *Overview of onset temperature determination for B-particles with concentration $x = 0.25$ at a pressure $P = 10.19$ for $N = 500$ particles: (a) $F_s(k,t)$ for selected temperatures around $T_o$ at $k = 5.4$; (b) derivatives $tF_s'(k,t)$ for the same temperatures as in (a); (c) Debye-Waller factor $f_s$ as function of $T$; (d) order parameter $\delta$ obtained from $tF_s'(k,t)$ as a function of $T$.*

In Figs. 7 to 10, we show results obtained for a larger system size $N = 8000$ and a much higher statistics than the one considered above and in the main text. Notice that the concentrations are different than those reported in Fig. 1 of the main text. As can be seen from the figure, the onset temperature obtained from a linear fit for $N = 8000$ is slightly lower than the one for $N = 500$. This is due to the temperature grid used in the $N = 8000$ simulations, which is coarser than for $N = 500$, and to the slight curvature of $\delta(T)$ for $N = 8000$ close to the onset temperature. These high-quality results confirm the presence of small oscillations at short times, which are visible also in Fig. 1 of the main text and will be further discussed in Sec. **??** below.

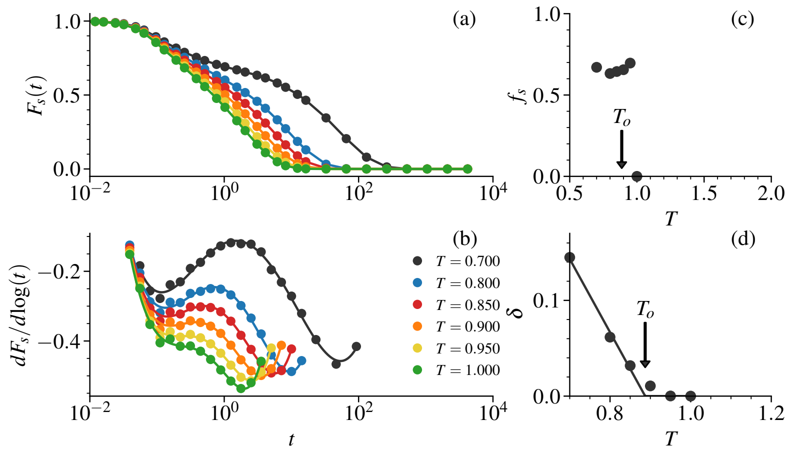


***Figure 7:*** *Overview of onset temperature determination for A-particles with concentration* $x = 0.18$ *at a pressure* $P = 10.19$ *for* $N = 8000$ *particles: (a)* $F_s(k,t)$ *for selected temperatures around* $T_o$ *at* $k = 7.2$*; (b) derivatives* $tF_s'(k,t)$ *for the same temperatures as in (a); (c) Debye-Waller factor* $f_s$ *as function of* $T$*; (d) order parameter* $\delta$ *obtained from* $tF_s'(k,t)$ *as a function of* $T$*.*

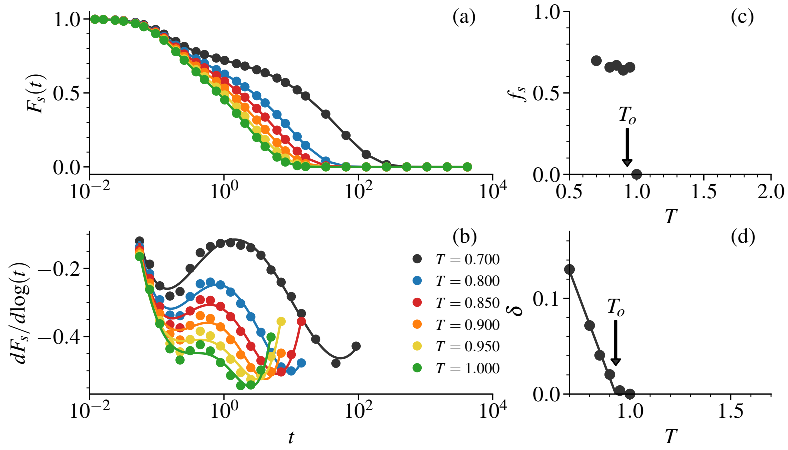


***Figure 8:*** *Overview of onset temperature determination for B-particles with concentration* $x = 0.18$ *at a pressure* $P = 10.19$ *for* $N = 8000$ *particles: (a)* $F_s(k,t)$ *for selected temperatures around* $T_o$ *at* $k = 5.4$*; (b) derivatives* $tF_s'(k,t)$ *for the same temperatures as in (a); (c) Debye-Waller factor* $f_s$ *as function of* $T$*; (d) order parameter* $\delta$ *obtained from* $tF_s'(k,t)$ *as a function of* $T$*.*

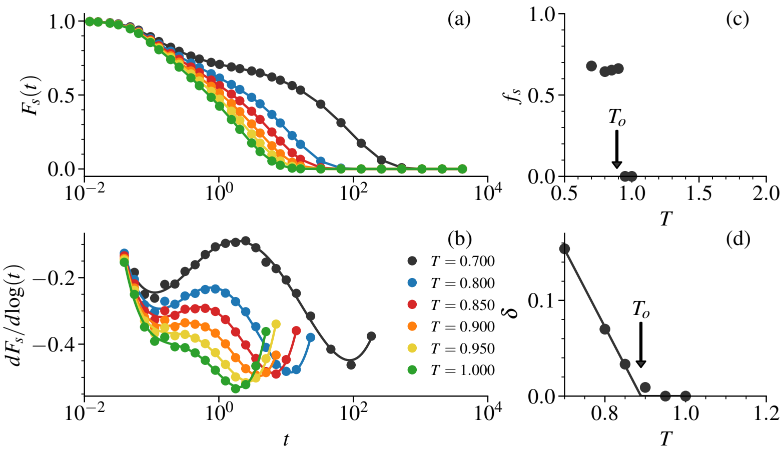


***Figure 9:*** *Overview of onset temperature determination for A-particles with concentration* $x = 0.26$ *at a pressure* $P = 10.19$ *for* $N = 8000$ *particles: (a)* $F_s(k,t)$ *for selected temperatures around* $T_o$ *at* $k = 7.2$*; (b) derivatives* $tF_s'(k,t)$ *for the same temperatures as in (a); (c) Debye-Waller factor* $f_s$ *as function of* $T$*; (d) order parameter* $\delta$ *obtained from* $tF_s'(k,t)$ *as a function of* $T$*.*

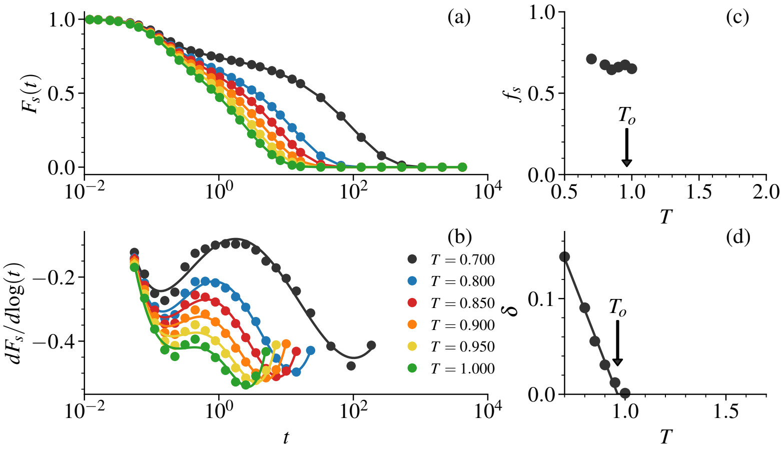


***Figure 10:*** *Overview of onset temperature determination for B-particles with concentration* $x = 0.26$ *at a pressure* $P = 10.19$ *for* $N = 8000$ *particles: (a)* $F_s(k,t)$ *for selected temperatures around* $T_o$ *at* $k = 5.6$*; (b) derivatives* $tF_s'(k,t)$ *for the same temperatures as in (a); (c) Debye-Waller factor* $f_s$ *as function of* $T$*; (d) order parameter* $\delta$ *obtained from* $tF_s'(k,t)$ *as a function of* $T$*.*

## 1.4 Comparison of the methods to determine the onset temperature

In this section we compare different methods to determine the onset temperatures:

- **linear fit** of the order parameter $\delta$, *i.e.,* the height of the smallest barrier separating the two minima of $tF_s'$, as a function of $T$: the onset temperature is defined as the temperature at which the linear fit reaches zero;
- **bracketing** of the temperature range across which $\delta$ jumps from 0 to a finite value: the onset temperature is then defined as the mid-point of that range.

From Fig. 11 we see that the results of the two methods are consistent within error bars. Note that error bars mostly reflect the spacing of the temperature grid around the onset temperature, see Sec. **??**.

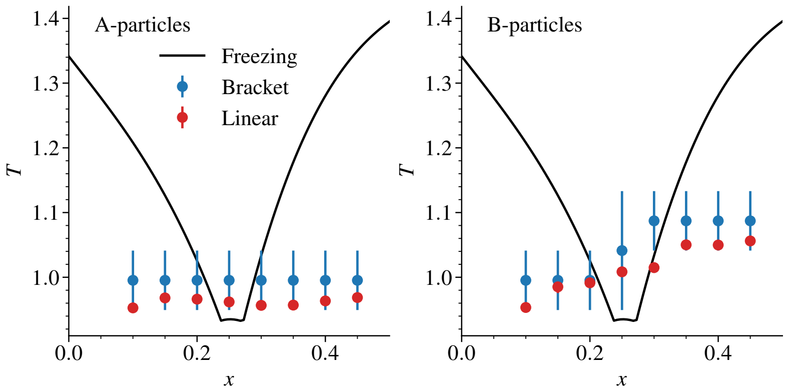


*Figure 11: Comparison of different methods to locate the onset: linear fit of $\delta(T)$ (red symbols) and bracketing method (blue symbols). Results are shown for A-particles at $k = 7.2$ (left) and B-particles at k=5.4 (right). The pressure is $P = 10.19$.*

## 1.5 Stability of the onset temperature against statistical noise

We now assess the robustness of the procedure to determine the onset temperature against statistical noise. To this end, we study how sensitive is $T_o$ to the number of independent trajectories over which the $F_s(k,t)$ are averaged. Namely, we use $M = 1, 2, 4, 8, 16, 30$ independent trajectories out of the 30 used to generate Fig. 1 of the main article. From Fig. 12, we see that the onset temperature converges very rapidly as a function of $M$: actually, within the statistical uncertainty of the fit, the results are representative of the large $M$ asymptote already with a single trajectory and already from $M = 2$ it is hard to see any change in $T_o$ when increasing the statistics.

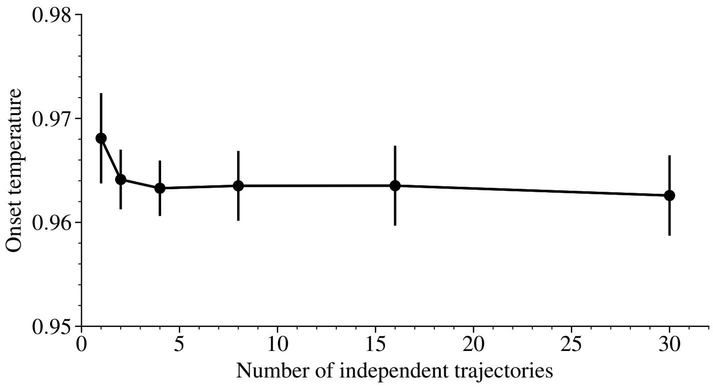


*Figure 12: Onset temperature, determined from the linear fit procedure, as a function of the number of independent trajectories used to compute the average $F_s(k,t)$.*

Note that, because of the nature of the fitting procedure used to determine $T_o$, the statistical uncertainty does not decrease with increasing $M$. The onset temperature determined using the bracketing procedure is also independent of $M$ (not shown). With both procedures, the only way to obtain a more precise estimate of the onset temperature is to use a finer temperature grid.

## 1.6 Composition-dependence of the onset temperature at different pressures

In Fig. 13, we compare the composition-dependence of the onset temperatures for A- and B-particles, at two different pressures: $P = 10.19$ and $P = 30$. The results are compared with the freezing points determined by Pedersen et al. [5]. The trends are qualitatively similar to those shown in Fig. 2 of the main text.

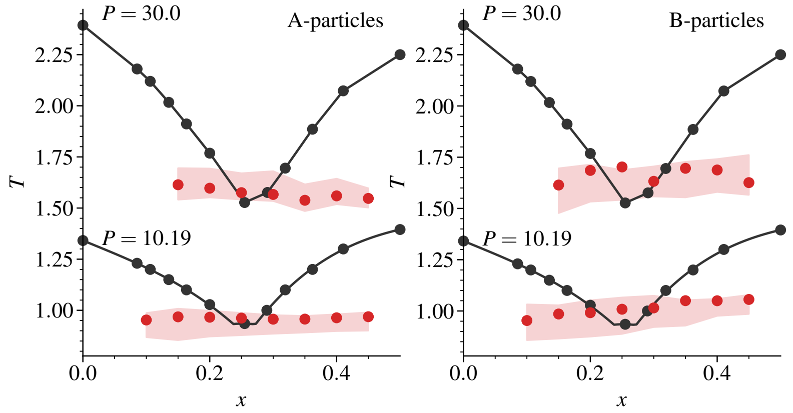


***Figure 13:*** *Freezing lines and onset temperatures for A-particles (left) and B-particles (right). Black circles indicate the freezing points determined by Pedersen et al. [5], red circles indicate the onset temperatures at $k = 7.4$ (for A-particles) and $k = 5.4$ (for B-particles). The shaded red areas indicate the range of onset temperatures corresponding to wavevectors between 5 and 10 for A-particles and in the range between 4 and 8 for B-particles, respectively.*

## 1.7 Structural relaxation times along isotherms

In Fig. 14, we show the structural relaxation times $\tau_\alpha$, computed separately for each species and determined from the decay to $1/e$ of the corresponding self intermediate scattering function, along several isotherms at constant pressure $P = 10.19$. We use the same value of $k$ for all state points in each given panel. We see that the relaxation times have a very mild dependence on concentration along isotherms. States at low temperature are not included for $x = 0.1$ because of partial crystallization.

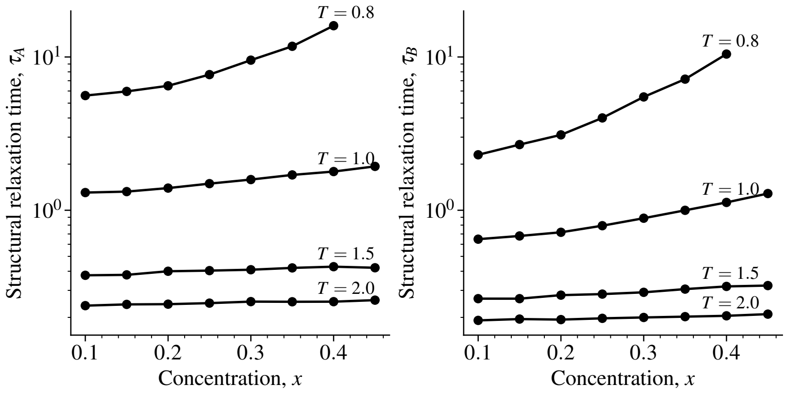


***Figure 14:*** *Structural relaxation times $\tau_\alpha$ as a function of $x$ for A- (left) and B-particles (right), evaluated at $k = 7.2$ and $k = 5.4$, respectively.*

### 1.8 Oscillatory behavior of $tF_s'$ at short times

To investigate the origin of the oscillations of the derivative $tF_s'(k,t)$ at short times, see Fig. 1 of the main text, we compare the simulation data with the Gaussian approximation

$$F_s(k,t) = \exp\left(-\frac{1}{6}k^2\delta r^2(t)\right),$$

where $\delta r^2(t)$ is the mean-square displacement. As usual, we consider A- and B-particles separately. Note that $\delta r^2(t)$ can be obtained also by integrating the velocity autocorrelation function $Z(t) = \frac{1}{3}\langle\vec{v}(t)\cdot\vec{v}(0)\rangle$. From Fig. 15 we see that the oscillations of $tF_s'(k,t)$ are well reproduced by the Gaussian approximation and correspond to those observed in $Z(t)$.

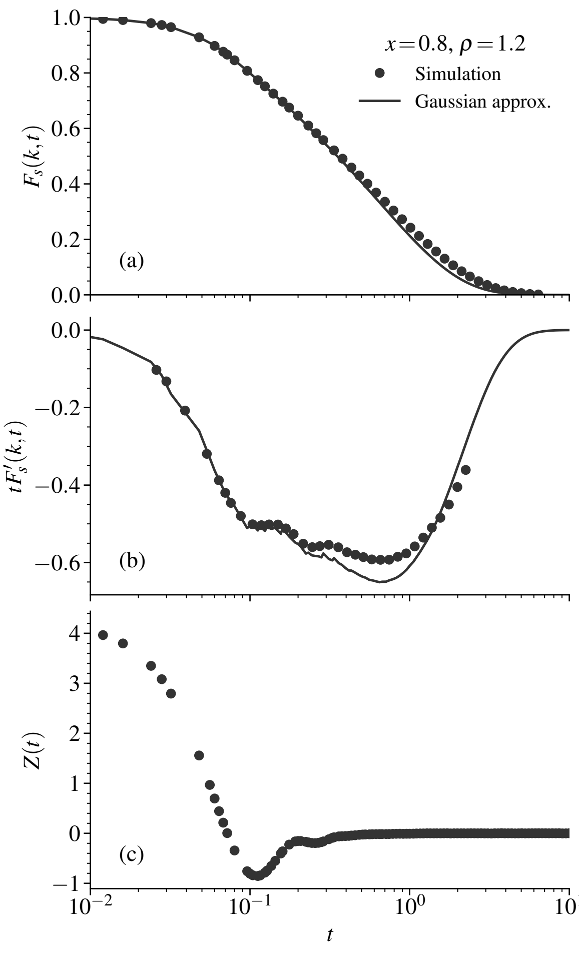


***Figure 15:*** *Analysis of short-time oscillations of the intermediate scattering functions at the state point ($T = 1.4$, $\rho = 1.2$) for the canonical concentration $x = 0.2$. (a) Self-inttermediate scattering function $F_s(k,t)$. (b) Derivative $tF_s'(k,t)$. (c) Velocity auto-correlation function $Z(t)$. The points are simulation data, the solid lines are predictions from the Gaussian approximation.*

We conclude that the fine structure of $tF_s'(k,t)$ at short times is neither a finite size effect, since similar oscillations are found also for $N = 8000$ (see for instance Fig. 7), nor an artifact due to statistical noise. They are a genuine physical feature characteristic of any dense liquid state of matter, unrelated to glassy dynamics. Indeed, we found in fact that the oscillations of $Z(t)$ persist over a broad range of temperature and density conditions, in agreement with previous work [6].

### 1.9 Excess entropy scaling of relaxation times and diffusion coeffients

We test the excess entropy scaling of the structural relaxation time and diffusion coefficients. We follow [7] and consider variables in appropriately reduced units. Note that for the calculation of $\tau_\alpha$ we keep a constant wave-vector $k$ in Lennard-Jones units, not in reduced units. Despite this minor discrepancy, the excess entropy scaling works pretty well, see Fig. 16. The excess entropy at the onset temperature is approximately constant, as indicated by the vertical lines.

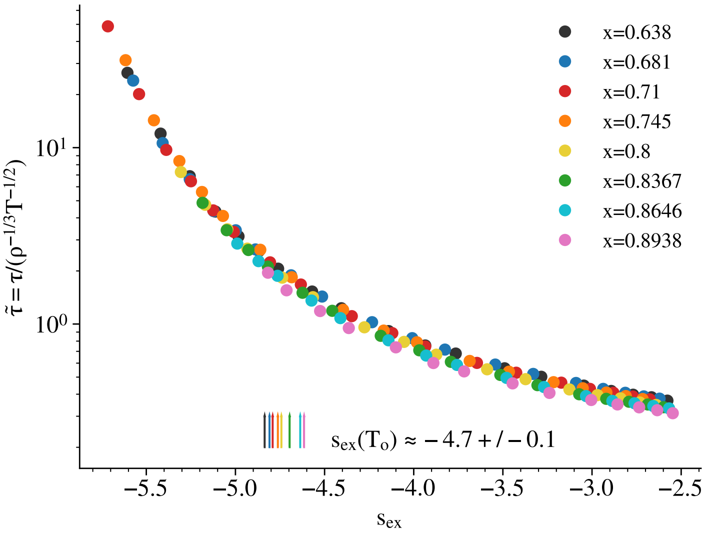


***Figure 16:*** *Reduced structural relaxation time $\tilde{\tau}$ for A-particles as a function of excess entropy $s_{ex}$ for different concentrations. The vertical lines mark the excess entropy at the onset temperature, which lines in the range between -4.8 and -4.6.*

We also perform an excess entropy scaling analysis for the reduced diffusion coefficient of the A-particles. These results are shown in Fig. 17 and show very good agreement with with the results of Bell *et al.* [7]. These findings further corroborate our analysis and might also indicate that the spread seen in Fig. 16 is due to the choice a fixed $k$.

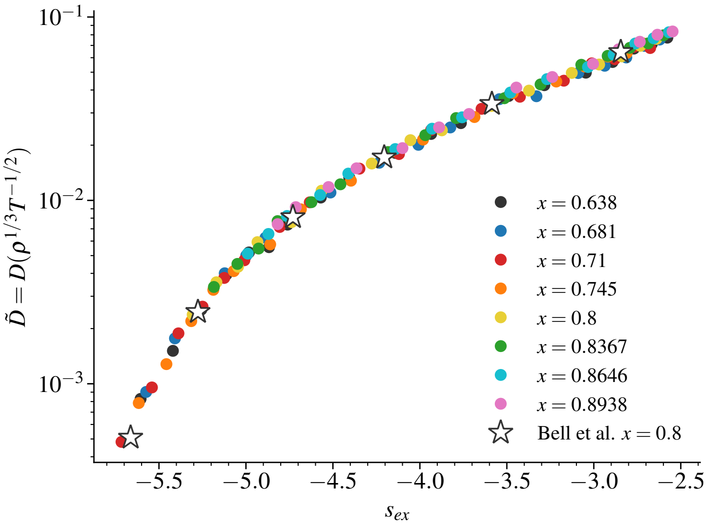


***Figure 17:*** *Reduced diffusion coefficient $\tilde{D}$ for A-particles as a function of excess entropy $s_{ex}$ for different concentrations. The results of Bell* et al. *[7] are included as stars.*

## 1.10 Tabulated data

To make it easier to quickly check our findings, we provide the values of the thermodynamic observables, the structural relaxation times $\tau_\alpha$ and the order parameters $\delta$ for the onset of glassiness corresponding to the simulations underlying Fig. 2 of the main text (system size N=500). Missing values are indicated with a dash and typically correspond to partly crystallized samples, which are excluded from the analysis.

***Table 1:*** *Thermodynamic data, structural relaxation times and order parameters for the onset of glassiness at different state points*

| | | | | A-particles | | | B-particles | | |
|---|---|---|---|---|---|---|---|---|---|
| $P$ | $x$ | $T$ | $\rho$ | $k$ | $\delta$ | $\tau_\alpha$ | $k$ | $\delta$ | $\tau_\alpha$ |
| 10.19 | 0.55 | 0.762 | 1.565 | 7.20 | – | $2.3\times10^{2}$ | 5.61 | – | $3.3\times10^{2}$ |
| 10.19 | 0.55 | 0.779 | 1.562 | 7.20 | – | $1.2\times10^{3}$ | 5.61 | – | $2.0\times10^{3}$ |
| 10.19 | 0.55 | 0.797 | 1.556 | 7.19 | 0.12 | $2.6\times10^{1}$ | 5.60 | 0.11 | $3.9\times10^{1}$ |
| 10.19 | 0.55 | 0.815 | 1.549 | 7.18 | – | $2.7\times10^{3}$ | 5.64 | – | $3.3\times10^{3}$ |
| 10.19 | 0.55 | 0.836 | 1.541 | 7.16 | 0.08 | $1.1\times10^{1}$ | 5.63 | 0.09 | $1.6\times10^{1}$ |
| 10.19 | 0.55 | 0.858 | 1.536 | 7.16 | 0.07 | $8.1\times10^{0}$ | 5.62 | 0.09 | $1.2\times10^{1}$ |
| 10.19 | 0.55 | 0.949 | 1.509 | 7.15 | 0.01 | $3.0\times10^{0}$ | 5.59 | 0.04 | $4.4\times10^{0}$ |
| 10.19 | 0.55 | 1.041 | 1.484 | 7.23 | 0.00 | $1.6\times10^{0}$ | 5.57 | 0.01 | $2.4\times10^{0}$ |
| 10.19 | 0.55 | 1.133 | 1.459 | 7.27 | 0.00 | $1.0\times10^{0}$ | 5.55 | 0.00 | $1.6\times10^{0}$ |
| 10.19 | 0.55 | 1.179 | 1.447 | 7.25 | 0.00 | $8.5\times10^{-1}$ | 5.54 | 0.00 | $1.3\times10^{0}$ |
| 10.19 | 0.55 | 1.225 | 1.436 | 7.23 | 0.00 | $7.5\times10^{-1}$ | 5.52 | 0.00 | $1.1\times10^{0}$ |
| 10.19 | 0.55 | 1.404 | 1.390 | 7.16 | 0.00 | $5.2\times10^{-1}$ | 5.66 | 0.00 | $6.7\times10^{-1}$ |
| 10.19 | 0.55 | 1.644 | 1.335 | 7.25 | 0.00 | $3.6\times10^{-1}$ | 5.61 | 0.00 | $4.7\times10^{-1}$ |
| 10.19 | 0.55 | 1.984 | 1.265 | 7.19 | 0.00 | $2.6\times10^{-1}$ | 5.61 | 0.00 | $3.4\times10^{-1}$ |
| 10.19 | 0.55 | 2.500 | 1.170 | 7.20 | 0.00 | $1.9\times10^{-1}$ | 5.61 | – | $2.5\times10^{-1}$ |
| 10.19 | 0.60 | 0.748 | 1.504 | 7.14 | 0.13 | $5.9\times10^{1}$ | 5.58 | 0.13 | $7.7\times10^{1}$ |
| 10.19 | 0.60 | 0.767 | 1.500 | 7.14 | 0.13 | $4.1\times10^{1}$ | 5.58 | 0.13 | $5.5\times10^{1}$ |

***Table 1:*** *Thermodynamic data, structural relaxation times and order parameters for the onset of glassiness at different state points – continued*

| | | | | A-particles | | | B-particles | | |
|---|---|---|---|---|---|---|---|---|---|
| $P$ | $x$ | $T$ | $\rho$ | $k$ | $\delta$ | $\tau_\alpha$ | $k$ | $\delta$ | $\tau_\alpha$ |
| 10.19 | 0.60 | 0.787 | 1.494 | 7.25 | 0.12 | $2.1\times10^{1}$ | 5.57 | 0.12 | $3.0\times10^{1}$ |
| 10.19 | 0.60 | 0.809 | 1.488 | 7.24 | 0.11 | $1.4\times10^{1}$ | 5.57 | 0.12 | $2.1\times10^{1}$ |
| 10.19 | 0.60 | 0.832 | 1.481 | 7.23 | 0.09 | $9.2\times10^{0}$ | 5.56 | 0.09 | $1.4\times10^{1}$ |
| 10.19 | 0.60 | 0.858 | 1.473 | 7.26 | 0.07 | $6.1\times10^{0}$ | 5.57 | 0.08 | $9.1\times10^{0}$ |
| 10.19 | 0.60 | 0.949 | 1.449 | 7.25 | 0.01 | $2.5\times10^{0}$ | 5.54 | 0.03 | $3.8\times10^{0}$ |
| 10.19 | 0.60 | 1.041 | 1.425 | 7.20 | 0.00 | $1.5\times10^{0}$ | 5.63 | 0.01 | $2.0\times10^{0}$ |
| 10.19 | 0.60 | 1.133 | 1.402 | 7.20 | 0.00 | $9.8\times10^{-1}$ | 5.67 | 0.00 | $1.3\times10^{0}$ |
| 10.19 | 0.60 | 1.179 | 1.391 | 7.17 | 0.00 | $8.6\times10^{-1}$ | 5.66 | 0.00 | $1.1\times10^{0}$ |
| 10.19 | 0.60 | 1.225 | 1.380 | 7.15 | 0.00 | $7.5\times10^{-1}$ | 5.64 | 0.00 | $9.8\times10^{-1}$ |
| 10.19 | 0.60 | 1.404 | 1.341 | 7.23 | 0.00 | $5.0\times10^{-1}$ | 5.62 | 0.00 | $6.5\times10^{-1}$ |
| 10.19 | 0.60 | 1.644 | 1.288 | 7.15 | 0.00 | $3.6\times10^{-1}$ | 5.52 | 0.00 | $4.7\times10^{-1}$ |
| 10.19 | 0.60 | 1.984 | 1.226 | 7.25 | 0.00 | $2.6\times10^{-1}$ | 5.61 | 0.00 | $3.3\times10^{-1}$ |
| 10.19 | 0.60 | 2.500 | 1.137 | 7.18 | 0.00 | $1.9\times10^{-1}$ | 5.57 | – | $2.5\times10^{-1}$ |
| 10.19 | 0.65 | 0.741 | 1.440 | 7.24 | 0.14 | $5.2\times10^{1}$ | 5.53 | 0.14 | $6.8\times10^{1}$ |
| 10.19 | 0.65 | 0.760 | 1.435 | 7.23 | 0.13 | $2.5\times10^{1}$ | 5.52 | 0.12 | $3.4\times10^{1}$ |
| 10.19 | 0.65 | 0.782 | 1.429 | 7.20 | 0.11 | $1.7\times10^{1}$ | 5.64 | 0.11 | $2.2\times10^{1}$ |
| 10.19 | 0.65 | 0.805 | 1.423 | 7.19 | 0.10 | $1.2\times10^{1}$ | 5.63 | 0.11 | $1.5\times10^{1}$ |
| 10.19 | 0.65 | 0.830 | 1.417 | 7.18 | 0.08 | $8.0\times10^{0}$ | 5.69 | 0.09 | $1.0\times10^{1}$ |
| 10.19 | 0.65 | 0.858 | 1.409 | 7.17 | 0.06 | $5.2\times10^{0}$ | 5.68 | 0.09 | $6.6\times10^{0}$ |
| 10.19 | 0.65 | 0.949 | 1.387 | 7.16 | 0.01 | $2.4\times10^{0}$ | 5.65 | 0.04 | $3.1\times10^{0}$ |
| 10.19 | 0.65 | 1.041 | 1.365 | 7.19 | 0.00 | $1.4\times10^{0}$ | 5.65 | 0.01 | $1.8\times10^{0}$ |
| 10.19 | 0.65 | 1.133 | 1.345 | 7.23 | 0.00 | $9.3\times10^{-1}$ | 5.62 | 0.00 | $1.2\times10^{0}$ |
| 10.19 | 0.65 | 1.179 | 1.335 | 7.25 | 0.00 | $8.1\times10^{-1}$ | 5.61 | 0.00 | $1.1\times10^{0}$ |
| 10.19 | 0.65 | 1.225 | 1.326 | 7.23 | 0.00 | $7.1\times10^{-1}$ | 5.60 | 0.00 | $9.3\times10^{-1}$ |
| 10.19 | 0.65 | 1.404 | 1.288 | 7.16 | 0.00 | $5.1\times10^{-1}$ | 5.52 | 0.00 | $6.5\times10^{-1}$ |
| 10.19 | 0.65 | 1.644 | 1.241 | 7.19 | 0.00 | $3.6\times10^{-1}$ | 5.58 | 0.00 | $4.4\times10^{-1}$ |
| 10.19 | 0.65 | 1.984 | 1.180 | 7.22 | 0.00 | $2.6\times10^{-1}$ | 5.63 | 0.00 | $3.2\times10^{-1}$ |
| 10.19 | 0.65 | 2.500 | 1.102 | 7.17 | 0.00 | $1.9\times10^{-1}$ | 5.56 | – | $2.4\times10^{-1}$ |
| 10.19 | 0.70 | 0.711 | 1.382 | 7.15 | 0.15 | $6.7\times10^{1}$ | 5.65 | 0.13 | $7.4\times10^{1}$ |
| 10.19 | 0.70 | 0.735 | 1.377 | 7.14 | 0.13 | $3.9\times10^{1}$ | 5.64 | 0.13 | $4.4\times10^{1}$ |
| 10.19 | 0.70 | 0.761 | 1.370 | 7.18 | 0.13 | $1.9\times10^{1}$ | 5.65 | 0.12 | $2.2\times10^{1}$ |
| 10.19 | 0.70 | 0.789 | 1.364 | 7.19 | 0.10 | $1.1\times10^{1}$ | 5.65 | 0.11 | $1.3\times10^{1}$ |
| 10.19 | 0.70 | 0.821 | 1.356 | 7.17 | 0.09 | $7.3\times10^{0}$ | 5.64 | 0.09 | $8.9\times10^{0}$ |
| 10.19 | 0.70 | 0.858 | 1.347 | 7.16 | 0.05 | $4.5\times10^{0}$ | 5.62 | 0.07 | $5.4\times10^{0}$ |
| 10.19 | 0.70 | 0.949 | 1.327 | 7.23 | 0.01 | $2.1\times10^{0}$ | 5.60 | 0.03 | $2.7\times10^{0}$ |
| 10.19 | 0.70 | 1.041 | 1.308 | 7.19 | 0.00 | $1.3\times10^{0}$ | 5.55 | 0.00 | $1.7\times10^{0}$ |
| 10.19 | 0.70 | 1.133 | 1.288 | 7.15 | 0.00 | $9.2\times10^{-1}$ | 5.52 | 0.00 | $1.2\times10^{0}$ |
| 10.19 | 0.70 | 1.179 | 1.278 | 7.22 | 0.00 | $7.9\times10^{-1}$ | 5.60 | 0.00 | $9.8\times10^{-1}$ |
| 10.19 | 0.70 | 1.225 | 1.270 | 7.20 | 0.00 | $7.0\times10^{-1}$ | 5.62 | 0.00 | $8.7\times10^{-1}$ |
| 10.19 | 0.70 | 1.404 | 1.236 | 7.18 | 0.00 | $4.9\times10^{-1}$ | 5.55 | 0.00 | $6.0\times10^{-1}$ |
| 10.19 | 0.70 | 1.644 | 1.193 | 7.23 | 0.00 | $3.5\times10^{-1}$ | 5.60 | 0.00 | $4.2\times10^{-1}$ |
| 10.19 | 0.70 | 1.984 | 1.137 | 7.18 | 0.00 | $2.6\times10^{-1}$ | 5.56 | – | $3.2\times10^{-1}$ |

***Table 1:*** *Thermodynamic data, structural relaxation times and order parameters for the onset of glassiness at different state points – continued*

| | | | | A-particles | | | B-particles | | |
|---|---|---|---|---|---|---|---|---|---|
| $P$ | $x$ | $T$ | $\rho$ | $k$ | $\delta$ | $\tau_\alpha$ | $k$ | $\delta$ | $\tau_\alpha$ |
| 10.19 | 0.70 | 2.500 | 1.063 | 7.24 | 0.00 | $1.9\times10^{-1}$ | 5.65 | – | $2.3\times10^{-1}$ |
| 10.19 | 0.75 | 0.728 | 1.315 | 7.20 | 0.14 | $2.6\times10^{1}$ | 5.56 | 0.12 | $2.9\times10^{1}$ |
| 10.19 | 0.75 | 0.755 | 1.309 | 7.19 | 0.11 | $1.5\times10^{1}$ | 5.55 | 0.11 | $1.7\times10^{1}$ |
| 10.19 | 0.75 | 0.785 | 1.303 | 7.18 | 0.10 | $9.7\times10^{0}$ | 5.54 | 0.10 | $1.1\times10^{1}$ |
| 10.19 | 0.75 | 0.819 | 1.295 | 7.17 | 0.08 | $6.3\times10^{0}$ | 5.53 | 0.07 | $7.1\times10^{0}$ |
| 10.19 | 0.75 | 0.858 | 1.288 | 7.15 | 0.06 | $4.1\times10^{0}$ | 5.52 | 0.06 | $4.9\times10^{0}$ |
| 10.19 | 0.75 | 0.949 | 1.269 | 7.20 | 0.01 | $2.0\times10^{0}$ | 5.62 | 0.03 | $2.4\times10^{0}$ |
| 10.19 | 0.75 | 1.041 | 1.251 | 7.21 | 0.00 | $1.2\times10^{0}$ | 5.59 | 0.00 | $1.5\times10^{0}$ |
| 10.19 | 0.75 | 1.133 | 1.234 | 7.17 | 0.00 | $8.8\times10^{-1}$ | 5.54 | 0.00 | $1.1\times10^{0}$ |
| 10.19 | 0.75 | 1.179 | 1.225 | 7.25 | 0.00 | $7.5\times10^{-1}$ | 5.61 | 0.00 | $9.1\times10^{-1}$ |
| 10.19 | 0.75 | 1.225 | 1.216 | 7.23 | 0.00 | $6.8\times10^{-1}$ | 5.60 | 0.00 | $8.1\times10^{-1}$ |
| 10.19 | 0.75 | 1.404 | 1.185 | 7.21 | 0.00 | $4.7\times10^{-1}$ | 5.64 | 0.00 | $5.6\times10^{-1}$ |
| 10.19 | 0.75 | 1.644 | 1.145 | 7.21 | 0.00 | $3.4\times10^{-1}$ | 5.58 | 0.00 | $4.1\times10^{-1}$ |
| 10.19 | 0.75 | 1.984 | 1.095 | 7.15 | 0.00 | $2.6\times10^{-1}$ | 5.55 | – | $3.1\times10^{-1}$ |
| 10.19 | 0.75 | 2.500 | 1.025 | 7.22 | 0.00 | $1.9\times10^{-1}$ | 5.63 | – | $2.3\times10^{-1}$ |
| 10.19 | 0.80 | 0.681 | 1.267 | 7.20 | 0.16 | $8.6\times10^{1}$ | 5.62 | 0.14 | $8.1\times10^{1}$ |
| 10.19 | 0.80 | 0.708 | 1.261 | 7.19 | 0.14 | $3.5\times10^{1}$ | 5.61 | 0.12 | $3.4\times10^{1}$ |
| 10.19 | 0.80 | 0.739 | 1.254 | 7.21 | 0.13 | $1.7\times10^{1}$ | 5.60 | 0.11 | $1.8\times10^{1}$ |
| 10.19 | 0.80 | 0.773 | 1.248 | 7.20 | 0.11 | $9.5\times10^{0}$ | 5.59 | 0.10 | $9.9\times10^{0}$ |
| 10.19 | 0.80 | 0.812 | 1.240 | 7.19 | 0.09 | $5.9\times10^{0}$ | 5.58 | 0.08 | $6.3\times10^{0}$ |
| 10.19 | 0.80 | 0.858 | 1.232 | 7.26 | 0.06 | $3.5\times10^{0}$ | 5.62 | 0.06 | $3.9\times10^{0}$ |
| 10.19 | 0.80 | 0.949 | 1.215 | 7.23 | 0.01 | $1.8\times10^{0}$ | 5.59 | 0.02 | $2.1\times10^{0}$ |
| 10.19 | 0.80 | 1.041 | 1.198 | 7.24 | 0.00 | $1.1\times10^{0}$ | 5.57 | 0.00 | $1.4\times10^{0}$ |
| 10.19 | 0.80 | 1.133 | 1.182 | 7.21 | 0.00 | $8.4\times10^{-1}$ | 5.63 | 0.00 | $9.7\times10^{-1}$ |
| 10.19 | 0.80 | 1.179 | 1.174 | 7.21 | 0.00 | $7.4\times10^{-1}$ | 5.62 | 0.00 | $8.4\times10^{-1}$ |
| 10.19 | 0.80 | 1.225 | 1.167 | 7.19 | 0.00 | $6.7\times10^{-1}$ | 5.61 | 0.00 | $7.6\times10^{-1}$ |
| 10.19 | 0.80 | 1.404 | 1.136 | 7.18 | 0.00 | $4.6\times10^{-1}$ | 5.56 | 0.00 | $5.5\times10^{-1}$ |
| 10.19 | 0.80 | 1.644 | 1.100 | 7.17 | 0.00 | $3.4\times10^{-1}$ | 5.56 | 0.00 | $4.0\times10^{-1}$ |
| 10.19 | 0.80 | 1.984 | 1.052 | 7.25 | 0.00 | $2.5\times10^{-1}$ | 5.68 | – | $3.0\times10^{-1}$ |
| 10.19 | 0.80 | 2.500 | 0.988 | 7.18 | 0.00 | $1.9\times10^{-1}$ | 5.58 | – | $2.3\times10^{-1}$ |
| 10.19 | 0.85 | 0.679 | 1.211 | 7.22 | 0.15 | $5.7\times10^{1}$ | 5.59 | 0.12 | $5.1\times10^{1}$ |
| 10.19 | 0.85 | 0.706 | 1.207 | 7.26 | 0.15 | $2.9\times10^{1}$ | 5.58 | 0.12 | $2.7\times10^{1}$ |
| 10.19 | 0.85 | 0.737 | 1.201 | 7.24 | 0.13 | $1.5\times10^{1}$ | 5.57 | 0.10 | $1.4\times10^{1}$ |
| 10.19 | 0.85 | 0.772 | 1.195 | 7.23 | 0.11 | $8.3\times10^{0}$ | 5.60 | 0.08 | $8.1\times10^{0}$ |
| 10.19 | 0.85 | 0.812 | 1.188 | 7.22 | 0.09 | $5.3\times10^{0}$ | 5.64 | 0.09 | $5.3\times10^{0}$ |
| 10.19 | 0.85 | 0.858 | 1.180 | 7.22 | 0.06 | $3.3\times10^{0}$ | 5.63 | 0.06 | $3.5\times10^{0}$ |
| 10.19 | 0.85 | 0.949 | 1.164 | 7.19 | 0.01 | $1.8\times10^{0}$ | 5.60 | 0.01 | $1.9\times10^{0}$ |
| 10.19 | 0.85 | 1.041 | 1.149 | 7.22 | 0.00 | $1.1\times10^{0}$ | 5.58 | 0.00 | $1.3\times10^{0}$ |
| 10.19 | 0.85 | 1.133 | 1.134 | 7.17 | 0.00 | $8.2\times10^{-1}$ | 5.56 | 0.00 | $9.4\times10^{-1}$ |
| 10.19 | 0.85 | 1.179 | 1.126 | 7.20 | 0.00 | $7.1\times10^{-1}$ | 5.55 | 0.00 | $8.3\times10^{-1}$ |
| 10.19 | 0.85 | 1.225 | 1.119 | 7.19 | 0.00 | $6.6\times10^{-1}$ | 5.53 | 0.00 | $7.6\times10^{-1}$ |
| 10.19 | 0.85 | 1.404 | 1.092 | 7.15 | 0.00 | $4.6\times10^{-1}$ | 5.54 | 0.00 | $5.3\times10^{-1}$ |

***Table 1:*** *Thermodynamic data, structural relaxation times and order parameters for the onset of glassiness at different state points – continued*

| | | | | A-particles | | | B-particles | | |
|---|---|---|---|---|---|---|---|---|---|
| $P$ | $x$ | $T$ | $\rho$ | $k$ | $\delta$ | $\tau_\alpha$ | $k$ | $\delta$ | $\tau_\alpha$ |
| 10.19 | 0.85 | 1.644 | 1.057 | 7.22 | 0.00 | $3.3\times10^{-1}$ | 5.64 | – | $3.8\times10^{-1}$ |
| 10.19 | 0.85 | 1.984 | 1.013 | 7.20 | 0.00 | $2.5\times10^{-1}$ | 5.62 | – | $3.0\times10^{-1}$ |
| 10.19 | 0.85 | 2.500 | 0.953 | 7.19 | 0.00 | $1.9\times10^{-1}$ | 5.58 | – | $2.3\times10^{-1}$ |
| 10.19 | 0.90 | 0.770 | – | 7.22 | – | – | 5.63 | – | – |
| 10.19 | 0.90 | 0.811 | 1.139 | 7.20 | 0.09 | $5.0\times10^{0}$ | 5.57 | 0.06 | $4.9\times10^{0}$ |
| 10.19 | 0.90 | 0.858 | 1.131 | 7.21 | 0.06 | $3.2\times10^{0}$ | 5.56 | 0.04 | $3.3\times10^{0}$ |
| 10.19 | 0.90 | 0.949 | 1.117 | 7.18 | 0.00 | $1.7\times10^{0}$ | 5.52 | 0.00 | $1.8\times10^{0}$ |
| 10.19 | 0.90 | 1.041 | 1.103 | 7.17 | 0.00 | $1.1\times10^{0}$ | 5.56 | 0.00 | $1.2\times10^{0}$ |
| 10.19 | 0.90 | 1.133 | 1.088 | 7.16 | 0.00 | $8.0\times10^{-1}$ | 5.63 | 0.00 | $8.6\times10^{-1}$ |
| 10.19 | 0.90 | 1.179 | 1.081 | 7.14 | 0.00 | $7.2\times10^{-1}$ | 5.61 | 0.00 | $7.6\times10^{-1}$ |
| 10.19 | 0.90 | 1.225 | 1.074 | 7.21 | 0.00 | $6.3\times10^{-1}$ | 5.67 | 0.00 | $6.8\times10^{-1}$ |
| 10.19 | 0.90 | 1.404 | 1.049 | 7.24 | 0.00 | $4.4\times10^{-1}$ | 5.67 | 0.00 | $4.8\times10^{-1}$ |
| 10.19 | 0.90 | 1.644 | 1.017 | 7.21 | 0.00 | $3.3\times10^{-1}$ | 5.63 | – | $3.8\times10^{-1}$ |
| 10.19 | 0.90 | 1.984 | 0.975 | 7.19 | 0.00 | $2.4\times10^{-1}$ | 5.58 | – | $3.0\times10^{-1}$ |
| 10.19 | 0.90 | 2.500 | 0.919 | 7.20 | 0.00 | $1.9\times10^{-1}$ | 5.64 | – | $2.3\times10^{-1}$ |
| 30.0 | 0.55 | 1.186 | 1.708 | 7.22 | – | $6.5\times10^{3}$ | 5.61 | – | $7.3\times10^{3}$ |
| 30.0 | 0.55 | 1.217 | 1.703 | 7.22 | 0.12 | $3.8\times10^{1}$ | 5.60 | 0.13 | $5.4\times10^{1}$ |
| 30.0 | 0.55 | 1.251 | 1.697 | 7.21 | – | $8.6\times10^{2}$ | 5.60 | – | $1.3\times10^{3}$ |
| 30.0 | 0.55 | 1.288 | 1.692 | 7.20 | 0.10 | $1.4\times10^{1}$ | 5.59 | 0.10 | $2.1\times10^{1}$ |
| 30.0 | 0.55 | 1.328 | 1.684 | 7.19 | 0.08 | $8.3\times10^{0}$ | 5.59 | 0.09 | $1.2\times10^{1}$ |
| 30.0 | 0.55 | 1.372 | 1.676 | 7.22 | 0.07 | $5.9\times10^{0}$ | 5.58 | 0.08 | $9.0\times10^{0}$ |
| 30.0 | 0.55 | 1.519 | 1.652 | 7.19 | 0.01 | $2.4\times10^{0}$ | 5.63 | 0.03 | $3.5\times10^{0}$ |
| 30.0 | 0.55 | 1.666 | 1.630 | 7.22 | 0.00 | $1.4\times10^{0}$ | 5.61 | 0.01 | $2.0\times10^{0}$ |
| 30.0 | 0.55 | 1.813 | 1.608 | 7.18 | 0.00 | $9.0\times10^{-1}$ | 5.58 | 0.00 | $1.3\times10^{0}$ |
| 30.0 | 0.55 | 1.887 | 1.598 | 7.24 | 0.00 | $7.5\times10^{-1}$ | 5.57 | 0.00 | $1.1\times10^{0}$ |
| 30.0 | 0.55 | 1.960 | 1.588 | 7.24 | 0.00 | $6.7\times10^{-1}$ | 5.64 | 0.00 | $9.6\times10^{-1}$ |
| 30.0 | 0.55 | 2.246 | 1.550 | 7.18 | 0.00 | $4.6\times10^{-1}$ | 5.64 | 0.00 | $6.1\times10^{-1}$ |
| 30.0 | 0.55 | 2.631 | 1.503 | 7.14 | 0.00 | $3.3\times10^{-1}$ | 5.58 | 0.00 | $4.3\times10^{-1}$ |
| 30.0 | 0.55 | 3.174 | 1.446 | 7.24 | 0.00 | $2.3\times10^{-1}$ | 5.54 | 0.00 | $3.1\times10^{-1}$ |
| 30.0 | 0.55 | 4.000 | 1.368 | 7.19 | 0.00 | $1.7\times10^{-1}$ | 5.65 | 0.00 | $2.1\times10^{-1}$ |
| 30.0 | 0.60 | 1.165 | 1.647 | 7.18 | 0.12 | $6.9\times10^{1}$ | 5.63 | 0.13 | $8.8\times10^{1}$ |
| 30.0 | 0.60 | 1.199 | 1.641 | 7.26 | 0.12 | $4.4\times10^{1}$ | 5.62 | 0.14 | $6.0\times10^{1}$ |
| 30.0 | 0.60 | 1.236 | 1.636 | 7.26 | 0.10 | $2.2\times10^{1}$ | 5.62 | 0.12 | $3.1\times10^{1}$ |
| 30.0 | 0.60 | 1.277 | 1.628 | 7.21 | 0.11 | $1.2\times10^{1}$ | 5.61 | 0.10 | $1.7\times10^{1}$ |
| 30.0 | 0.60 | 1.322 | 1.622 | 7.20 | 0.08 | $7.8\times10^{0}$ | 5.60 | 0.09 | $1.1\times10^{1}$ |
| 30.0 | 0.60 | 1.372 | 1.614 | 7.19 | 0.06 | $5.1\times10^{0}$ | 5.59 | 0.08 | $7.4\times10^{0}$ |
| 30.0 | 0.60 | 1.519 | 1.592 | 7.24 | 0.01 | $2.3\times10^{0}$ | 5.64 | 0.04 | $3.2\times10^{0}$ |
| 30.0 | 0.60 | 1.666 | 1.571 | 7.21 | 0.00 | $1.3\times10^{0}$ | 5.62 | 0.01 | $1.9\times10^{0}$ |
| 30.0 | 0.60 | 1.813 | 1.552 | 7.18 | 0.00 | $9.0\times10^{-1}$ | 5.64 | 0.00 | $1.2\times10^{0}$ |
| 30.0 | 0.60 | 1.887 | 1.541 | 7.16 | 0.00 | $7.7\times10^{-1}$ | 5.63 | 0.00 | $1.0\times10^{0}$ |
| 30.0 | 0.60 | 1.960 | 1.531 | 7.16 | 0.00 | $6.9\times10^{-1}$ | 5.62 | 0.00 | $9.0\times10^{-1}$ |
| 30.0 | 0.60 | 2.246 | 1.497 | 7.13 | 0.00 | $4.7\times10^{-1}$ | 5.57 | 0.00 | $6.1\times10^{-1}$ |

***Table 1:*** *Thermodynamic data, structural relaxation times and order parameters for the onset of glassiness at different state points – continued*

| | | | | A-particles | | | B-particles | | |
|---|---|---|---|---|---|---|---|---|---|
| $P$ | $x$ | $T$ | $\rho$ | $k$ | $\delta$ | $\tau_\alpha$ | $k$ | $\delta$ | $\tau_\alpha$ |
| 30.0 | 0.60 | 2.631 | 1.455 | 7.26 | 0.00 | $3.2\times10^{-1}$ | 5.55 | 0.00 | $4.2\times10^{-1}$ |
| 30.0 | 0.60 | 3.174 | 1.401 | 7.20 | 0.00 | $2.4\times10^{-1}$ | 5.67 | 0.00 | $2.8\times10^{-1}$ |
| 30.0 | 0.60 | 4.000 | 1.328 | 7.23 | 0.00 | $1.7\times10^{-1}$ | 5.60 | 0.00 | $2.1\times10^{-1}$ |
| 30.0 | 0.65 | 1.164 | 1.581 | 7.23 | 0.14 | $6.5\times10^{1}$ | 5.63 | 0.13 | $8.0\times10^{1}$ |
| 30.0 | 0.65 | 1.199 | 1.575 | 7.22 | 0.12 | $3.2\times10^{1}$ | 5.62 | 0.14 | $4.0\times10^{1}$ |
| 30.0 | 0.65 | 1.236 | 1.570 | 7.21 | 0.12 | $1.7\times10^{1}$ | 5.61 | 0.11 | $2.2\times10^{1}$ |
| 30.0 | 0.65 | 1.277 | 1.564 | 7.20 | 0.11 | $1.1\times10^{1}$ | 5.61 | 0.11 | $1.5\times10^{1}$ |
| 30.0 | 0.65 | 1.322 | 1.558 | 7.19 | 0.08 | $6.9\times10^{0}$ | 5.60 | 0.09 | $8.9\times10^{0}$ |
| 30.0 | 0.65 | 1.372 | 1.550 | 7.18 | 0.06 | $4.8\times10^{0}$ | 5.64 | 0.08 | $6.3\times10^{0}$ |
| 30.0 | 0.65 | 1.519 | 1.530 | 7.15 | 0.01 | $2.2\times10^{0}$ | 5.61 | 0.04 | $2.9\times10^{0}$ |
| 30.0 | 0.65 | 1.666 | 1.511 | 7.15 | 0.00 | $1.3\times10^{0}$ | 5.59 | 0.01 | $1.7\times10^{0}$ |
| 30.0 | 0.65 | 1.813 | 1.493 | 7.24 | 0.00 | $8.6\times10^{-1}$ | 5.57 | 0.00 | $1.2\times10^{0}$ |
| 30.0 | 0.65 | 1.887 | 1.484 | 7.23 | 0.00 | $7.5\times10^{-1}$ | 5.57 | 0.00 | $1.0\times10^{0}$ |
| 30.0 | 0.65 | 1.960 | 1.475 | 7.27 | 0.00 | $6.4\times10^{-1}$ | 5.57 | 0.00 | $8.8\times10^{-1}$ |
| 30.0 | 0.65 | 2.246 | 1.444 | 7.24 | 0.00 | $4.5\times10^{-1}$ | 5.53 | 0.00 | $6.0\times10^{-1}$ |
| 30.0 | 0.65 | 2.631 | 1.404 | 7.20 | 0.00 | $3.2\times10^{-1}$ | 5.68 | 0.00 | $3.9\times10^{-1}$ |
| 30.0 | 0.65 | 3.174 | 1.354 | 7.17 | 0.00 | $2.4\times10^{-1}$ | 5.63 | 0.00 | $2.8\times10^{-1}$ |
| 30.0 | 0.65 | 4.000 | 1.287 | 7.15 | 0.00 | $1.7\times10^{-1}$ | 5.52 | 0.00 | $2.2\times10^{-1}$ |
| 30.0 | 0.70 | 1.118 | 1.521 | 7.14 | 0.14 | $1.2\times10^{2}$ | 5.60 | 0.15 | $1.2\times10^{2}$ |
| 30.0 | 0.70 | 1.158 | 1.516 | 7.13 | 0.13 | $4.2\times10^{1}$ | 5.60 | 0.14 | $4.6\times10^{1}$ |
| 30.0 | 0.70 | 1.203 | 1.509 | 7.15 | 0.12 | $2.2\times10^{1}$ | 5.59 | 0.14 | $2.5\times10^{1}$ |
| 30.0 | 0.70 | 1.253 | 1.504 | 7.14 | 0.10 | $1.3\times10^{1}$ | 5.58 | 0.10 | $1.5\times10^{1}$ |
| 30.0 | 0.70 | 1.309 | 1.496 | 7.25 | 0.08 | $6.9\times10^{0}$ | 5.57 | 0.10 | $8.8\times10^{0}$ |
| 30.0 | 0.70 | 1.372 | 1.488 | 7.24 | 0.06 | $4.4\times10^{0}$ | 5.57 | 0.08 | $5.6\times10^{0}$ |
| 30.0 | 0.70 | 1.519 | 1.470 | 7.26 | 0.01 | $2.1\times10^{0}$ | 5.57 | 0.03 | $2.6\times10^{0}$ |
| 30.0 | 0.70 | 1.666 | 1.452 | 7.26 | 0.00 | $1.3\times10^{0}$ | 5.54 | 0.01 | $1.6\times10^{0}$ |
| 30.0 | 0.70 | 1.813 | 1.436 | 7.23 | 0.00 | $8.7\times10^{-1}$ | 5.52 | 0.00 | $1.1\times10^{0}$ |
| 30.0 | 0.70 | 1.887 | 1.427 | 7.20 | 0.00 | $7.6\times10^{-1}$ | 5.64 | 0.00 | $9.2\times10^{-1}$ |
| 30.0 | 0.70 | 1.960 | 1.419 | 7.19 | 0.00 | $6.7\times10^{-1}$ | 5.70 | 0.00 | $7.8\times10^{-1}$ |
| 30.0 | 0.70 | 2.246 | 1.390 | 7.16 | 0.00 | $4.6\times10^{-1}$ | 5.66 | 0.00 | $5.4\times10^{-1}$ |
| 30.0 | 0.70 | 2.631 | 1.353 | 7.17 | 0.00 | $3.3\times10^{-1}$ | 5.63 | 0.00 | $3.8\times10^{-1}$ |
| 30.0 | 0.70 | 3.174 | 1.307 | 7.19 | 0.00 | $2.3\times10^{-1}$ | 5.55 | 0.00 | $2.8\times10^{-1}$ |
| 30.0 | 0.70 | 4.000 | 1.245 | 7.19 | 0.00 | $1.7\times10^{-1}$ | 5.58 | 0.00 | $2.1\times10^{-1}$ |
| 30.0 | 0.75 | 1.132 | 1.457 | 7.26 | 0.15 | $5.3\times10^{1}$ | 5.55 | 0.13 | $5.6\times10^{1}$ |
| 30.0 | 0.75 | 1.170 | 1.452 | 7.25 | 0.13 | $3.0\times10^{1}$ | 5.54 | 0.13 | $3.2\times10^{1}$ |
| 30.0 | 0.75 | 1.213 | 1.447 | 7.25 | 0.12 | $1.6\times10^{1}$ | 5.54 | 0.12 | $1.9\times10^{1}$ |
| 30.0 | 0.75 | 1.260 | 1.441 | 7.24 | 0.12 | $1.0\times10^{1}$ | 5.53 | 0.12 | $1.1\times10^{1}$ |
| 30.0 | 0.75 | 1.313 | 1.434 | 7.22 | 0.08 | $6.1\times10^{0}$ | 5.52 | 0.08 | $7.0\times10^{0}$ |
| 30.0 | 0.75 | 1.372 | 1.428 | 7.20 | 0.07 | $4.2\times10^{0}$ | 5.64 | 0.08 | $4.6\times10^{0}$ |
| 30.0 | 0.75 | 1.519 | 1.412 | 7.17 | 0.02 | $2.1\times10^{0}$ | 5.69 | 0.04 | $2.3\times10^{0}$ |
| 30.0 | 0.75 | 1.666 | 1.396 | 7.17 | 0.00 | $1.3\times10^{0}$ | 5.66 | 0.01 | $1.4\times10^{0}$ |
| 30.0 | 0.75 | 1.813 | 1.380 | 7.15 | 0.00 | $9.0\times10^{-1}$ | 5.64 | 0.00 | $1.0\times10^{0}$ |

***Table 1:*** *Thermodynamic data, structural relaxation times and order parameters for the onset of glassiness at different state points – continued*

| | | | | A-particles | | | B-particles | | |
|---|---|---|---|---|---|---|---|---|---|
| $P$ | $x$ | $T$ | $\rho$ | $k$ | $\delta$ | $\tau_\alpha$ | $k$ | $\delta$ | $\tau_\alpha$ |
| 30.0 | 0.75 | 1.887 | 1.373 | 7.19 | 0.00 | $7.6\times10^{-1}$ | 5.63 | 0.00 | $8.7\times10^{-1}$ |
| 30.0 | 0.75 | 1.960 | 1.366 | 7.19 | 0.00 | $6.7\times10^{-1}$ | 5.65 | 0.00 | $7.6\times10^{-1}$ |
| 30.0 | 0.75 | 2.246 | 1.339 | 7.25 | 0.00 | $4.5\times10^{-1}$ | 5.61 | 0.00 | $5.3\times10^{-1}$ |
| 30.0 | 0.75 | 2.631 | 1.304 | 7.18 | 0.00 | $3.2\times10^{-1}$ | 5.55 | 0.00 | $3.8\times10^{-1}$ |
| 30.0 | 0.75 | 3.174 | 1.261 | 7.19 | 0.00 | $2.3\times10^{-1}$ | 5.61 | 0.00 | $2.7\times10^{-1}$ |
| 30.0 | 0.75 | 4.000 | 1.203 | 7.25 | 0.00 | $1.7\times10^{-1}$ | 5.58 | 0.00 | $2.1\times10^{-1}$ |
| 30.0 | 0.80 | 1.096 | 1.401 | 7.20 | 0.15 | $1.1\times10^{2}$ | 5.67 | 0.14 | $8.8\times10^{1}$ |
| 30.0 | 0.80 | 1.139 | 1.396 | 7.17 | 0.14 | $4.0\times10^{1}$ | 5.67 | 0.13 | $3.6\times10^{1}$ |
| 30.0 | 0.80 | 1.187 | 1.391 | 7.16 | 0.12 | $2.0\times10^{1}$ | 5.66 | 0.12 | $1.8\times10^{1}$ |
| 30.0 | 0.80 | 1.241 | 1.385 | 7.15 | 0.10 | $1.1\times10^{1}$ | 5.65 | 0.12 | $1.0\times10^{1}$ |
| 30.0 | 0.80 | 1.302 | 1.379 | 7.14 | 0.10 | $6.7\times10^{0}$ | 5.64 | 0.10 | $6.5\times10^{0}$ |
| 30.0 | 0.80 | 1.372 | 1.371 | 7.19 | 0.07 | $4.1\times10^{0}$ | 5.64 | 0.08 | $4.1\times10^{0}$ |
| 30.0 | 0.80 | 1.519 | 1.357 | 7.17 | 0.02 | $2.1\times10^{0}$ | 5.64 | 0.03 | $2.2\times10^{0}$ |
| 30.0 | 0.80 | 1.666 | 1.342 | 7.23 | 0.00 | $1.2\times10^{0}$ | 5.62 | 0.01 | $1.4\times10^{0}$ |
| 30.0 | 0.80 | 1.813 | 1.328 | 7.23 | 0.00 | $8.6\times10^{-1}$ | 5.60 | 0.00 | $9.8\times10^{-1}$ |
| 30.0 | 0.80 | 1.887 | 1.320 | 7.22 | 0.00 | $7.5\times10^{-1}$ | 5.57 | 0.00 | $8.6\times10^{-1}$ |
| 30.0 | 0.80 | 1.960 | 1.313 | 7.20 | 0.00 | $6.7\times10^{-1}$ | 5.56 | 0.00 | $7.5\times10^{-1}$ |
| 30.0 | 0.80 | 2.246 | 1.289 | 7.16 | 0.00 | $4.6\times10^{-1}$ | 5.53 | 0.00 | $5.3\times10^{-1}$ |
| 30.0 | 0.80 | 2.631 | 1.257 | 7.22 | 0.00 | $3.2\times10^{-1}$ | 5.60 | 0.00 | $3.6\times10^{-1}$ |
| 30.0 | 0.80 | 3.174 | 1.218 | 7.23 | 0.00 | $2.3\times10^{-1}$ | 5.60 | 0.00 | $2.7\times10^{-1}$ |
| 30.0 | 0.80 | 4.000 | 1.161 | 7.18 | 0.00 | $1.7\times10^{-1}$ | 5.60 | 0.00 | $2.0\times10^{-1}$ |
| 30.0 | 0.85 | 1.119 | 1.344 | 7.23 | 0.15 | $6.2\times10^{1}$ | 5.62 | 0.13 | $4.8\times10^{1}$ |
| 30.0 | 0.85 | 1.146 | 1.340 | 7.22 | 0.14 | $3.8\times10^{1}$ | 5.61 | 0.14 | $3.1\times10^{1}$ |
| 30.0 | 0.85 | 1.159 | 1.339 | 7.22 | 0.14 | $3.1\times10^{1}$ | 5.61 | 0.13 | $2.5\times10^{1}$ |
| 30.0 | 0.85 | 1.183 | 1.337 | 7.25 | 0.13 | $2.2\times10^{1}$ | 5.61 | 0.13 | $1.9\times10^{1}$ |
| 30.0 | 0.85 | 1.204 | 1.334 | 7.25 | 0.12 | $1.5\times10^{1}$ | 5.61 | 0.11 | $1.4\times10^{1}$ |
| 30.0 | 0.85 | 1.223 | 1.333 | 7.24 | 0.13 | $1.3\times10^{1}$ | 5.60 | 0.12 | $1.2\times10^{1}$ |
| 30.0 | 0.85 | 1.253 | 1.330 | 7.24 | 0.12 | $9.6\times10^{0}$ | 5.60 | 0.09 | $8.8\times10^{0}$ |
| 30.0 | 0.85 | 1.267 | 1.328 | 7.23 | 0.12 | $8.4\times10^{0}$ | 5.60 | 0.09 | $7.8\times10^{0}$ |
| 30.0 | 0.85 | 1.309 | 1.324 | 7.23 | 0.10 | $6.2\times10^{0}$ | 5.60 | 0.10 | $5.8\times10^{0}$ |
| 30.0 | 0.85 | 1.317 | 1.323 | 7.23 | 0.09 | $5.8\times10^{0}$ | 5.57 | 0.10 | $5.6\times10^{0}$ |
| 30.0 | 0.85 | 1.372 | 1.318 | 7.22 | 0.08 | $4.0\times10^{0}$ | 5.57 | 0.07 | $4.0\times10^{0}$ |
| 30.0 | 0.85 | 1.519 | 1.304 | 7.18 | 0.02 | $2.0\times10^{0}$ | 5.55 | 0.02 | $2.1\times10^{0}$ |
| 30.0 | 0.85 | 1.666 | 1.291 | 7.16 | 0.00 | $1.3\times10^{0}$ | 5.53 | 0.00 | $1.4\times10^{0}$ |
| 30.0 | 0.85 | 1.813 | 1.278 | 7.22 | 0.00 | $8.7\times10^{-1}$ | 5.60 | 0.00 | $9.4\times10^{-1}$ |
| 30.0 | 0.85 | 1.887 | 1.271 | 7.21 | 0.00 | $7.5\times10^{-1}$ | 5.62 | 0.00 | $8.0\times10^{-1}$ |
| 30.0 | 0.85 | 1.960 | 1.265 | 7.19 | 0.00 | $6.7\times10^{-1}$ | 5.61 | 0.00 | $7.2\times10^{-1}$ |
| 30.0 | 0.85 | 2.246 | 1.241 | 7.19 | 0.00 | $4.5\times10^{-1}$ | 5.58 | 0.00 | $5.0\times10^{-1}$ |
| 30.0 | 0.85 | 2.631 | 1.212 | 7.22 | 0.00 | $3.2\times10^{-1}$ | 5.59 | 0.00 | $3.6\times10^{-1}$ |
| 30.0 | 0.85 | 3.174 | 1.174 | 7.21 | 0.00 | $2.3\times10^{-1}$ | 5.62 | 0.00 | $2.6\times10^{-1}$ |
| 30.0 | 0.85 | 4.000 | 1.124 | 7.20 | 0.00 | $1.7\times10^{-1}$ | 5.54 | 0.00 | $2.0\times10^{-1}$ |

# References

[1] D. Coslovich. "atooms: A framework for simulations of interacting particles (3.22.0)." (2017–2024). URL http://dx.doi.org/10.5281/zenodo.1183301.

[2] S. Nose. J. Phys. Soc. Jap., **70**, 75 (2001). URL http://dx.doi.org/10.1143/JPSJ.70.75.

[3] N. Bailey, J. S. Hansen, T. Ingebrigtsen, *et al.* SciPost Phys., **3**, 038 (2017). URL http://dx.doi.org/10.21468/SciPostPhys.3.6.038.

[4] G. J. Martyna, D. J. Tobias, and M. L. Klein. J. Chem. Phys., **101**, 4177 (1994). URL http://dx.doi.org/10.1063/1.467468.

[5] U. R. Pedersen, T. B. Schrøder, and J. C. Dyre. Phys. Rev. Lett., **120**, 165501 (2018). URL http://dx.doi.org/10.1103/PhysRevLett.120.165501.

[6] V. V. Brazhkin, Y. D. Fomin, A. G. Lyapin, *et al.* Phys. Rev. Lett., **111**, 145901 (2013). URL http://dx.doi.org/10.1103/PhysRevLett.111.145901.

[7] I. H. Bell, J. C. Dyre, and T. S. Ingebrigtsen. Nat. Commun., **11**, 4300 (2020). URL http://dx.doi.org/10.1038/s41467-020-17948-1.
